# Supplementary material for: Improved Analysis of EDCS via Gallai-Edmonds Decomposition
Source: arXiv:2110.05746 source file (2021-10-12)
Supplement: Supplementary file 1 [file appendix.tex]

%\section{Tutte-Berge Characterization of Maximum Matching}\label{sec:appendix}
%
%In this section, we present the proof of \Cref{lem:tutte-berg-char}.

%\begin{proof}[Proof of \Cref{lem:tutte-berg-char}]
%	Call a component $C_i$ {\em perfect} if all of its vertices are matched by $M$ (not necessarily together) and {\em imperfect} otherwise. The vertices of an odd size component $C_i$ clearly cannot be all matched together due to parity. As such, any perfect odd size component $C_i$ has a vertex $v_i$ that is matched to a vertex $u_i \not\in C_i$ and since $C_i$ is a connected component of $G - U$, $u_i$ must belong to $U$. Since every vertex of $U$ is matched to at most one other vertex in $M$, the number of perfect odd size components is upper bounded by $|U|$.
%	
%	Now observe from \Cref{prop:tutte} that $M$ must match $n + |U| - \odd(G - U)$ vertices. As such, at most $n - (n + |U| - \odd(G - U)) = \odd(G - U) - |U|$ vertices are left unmatched by $M$; this is also clearly an upper bound on the number of imperfect odd size components. Hence, the number of perfect odd size components must be at least $\odd(G-U) - (\odd(G-U) - |U|) = |U|$. 
%	
%	The two upper and lower bounds above on the number of perfect odd size components, imply together that the number of perfect odd components must be exactly $|U|$. From our discussion above that every perfect odd size component has at least a vertex matched to $U$, we thus get that every vertex of $U$ must be matched to a unique perfect odd size component, proving property (3). Furthermore, all the rest of vertices not matched to $U$ must be matched inside the components $C_1, \ldots, C_k$ since there are no edges between two components $C_i$ and $C_j$.
%	
%	To finish the proof of properties (1) and (2), note that since the number of perfect odd size components is exactly $|U|$, the number of imperfect odd size components is exactly $\odd(H - U) - |U|$. Given that the total number of vertices left unmatched by $M$ is at most $\odd(H - U) - |U|$ as shown above, we get that every imperfect odd size component has exactly one vertex unmatched by $M$ and these are all the vertices left unmatched by $M$.
%\end{proof}
